# Supplementary material for: Learning Long-form Video Prior via Generative Pre-Training
Source: arXiv:2404.15909 source file (2024-04-24)
Supplement: Supplementary file 1 [file supp_dataset.pdf]

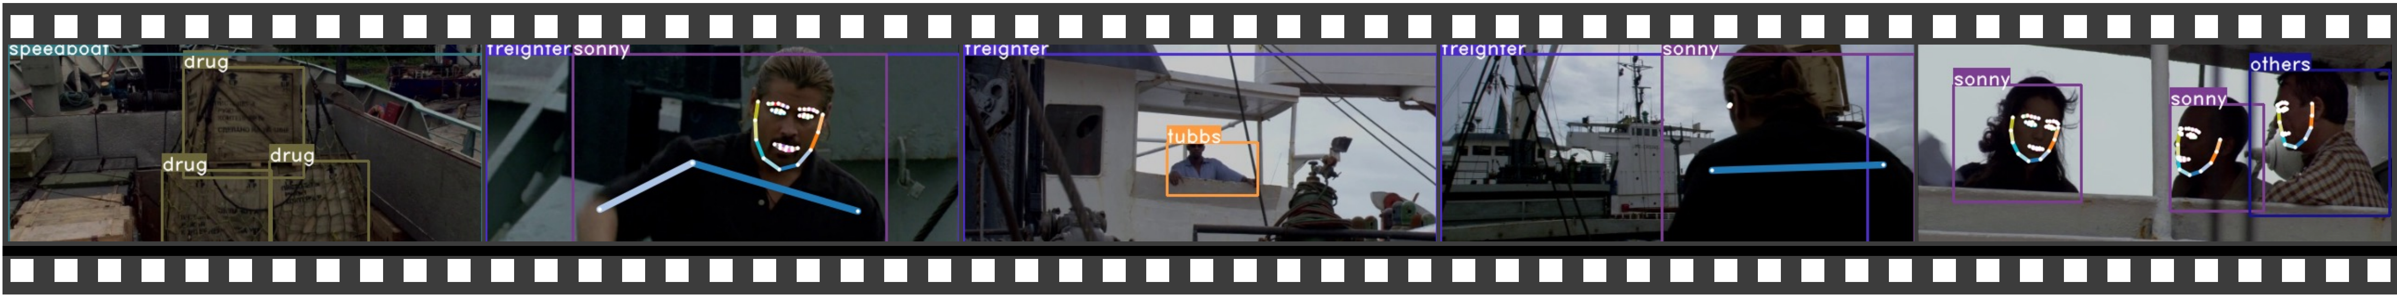


Scripts (condensed):

Sonny and Tubbs and the rest of the squad (except Trudy) begin loading drugs from a freighter onto some speedboats.

Summative annotations:
Title: “undercover operation: sonny and tubbs' drug seizure”
Genre: “'crime and action”
Emotion: “'determination and focus”
Scene: “'freighter and speedboats”
Summary: “'sonny, tubbs, and the rest of the squad embark on a risky operation to seize drugs from a freighter”

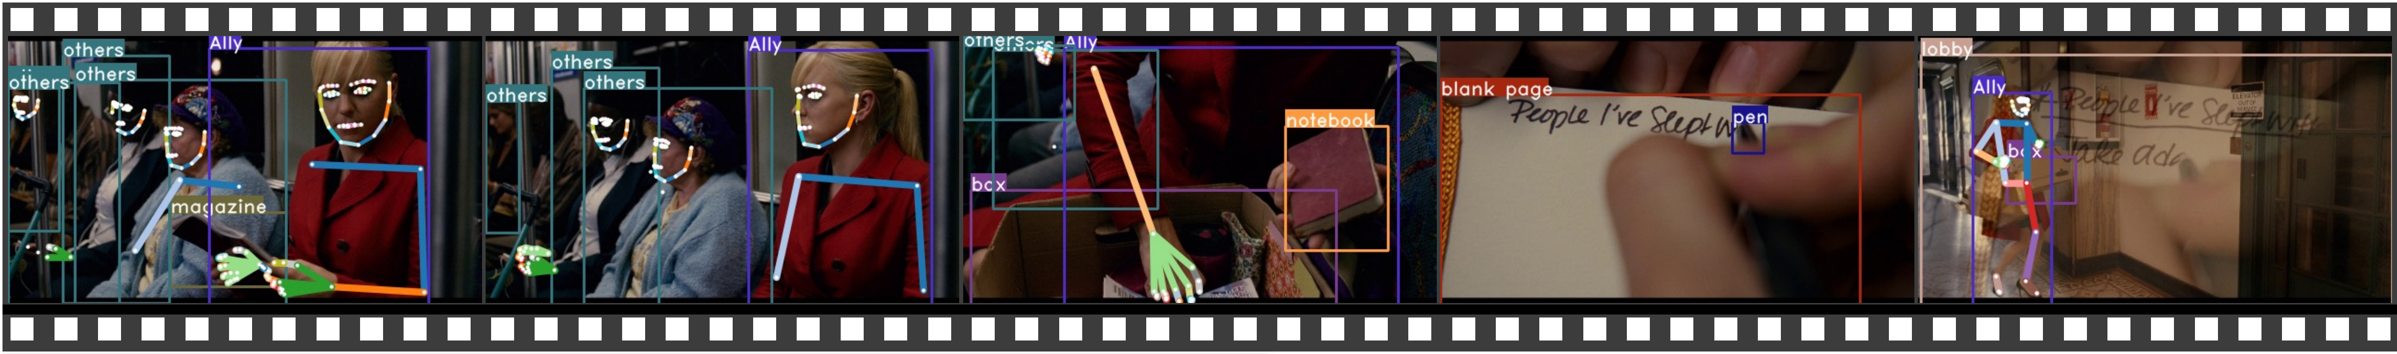


Scripts (shot by shot):
(1) Ally sets the magazine aside.
(2) then bites her lip and shifts her calculating gaze.
(3) Ally reaches into the box and pulls out a small notebook and pen.
(4) Glancing around, Ally opens it and heads a blank page with the words “People I’ve Slept With”.
(5) Now as Ally enters her apartment building's lobby, her list fades into view.

Summative annotations:
Title: “intimate confessions”
Genre: “'drama and introspective”
Emotion: “calculating, contemplative, vulnerable, and secretive”
Scene: “apartment building lobby”
Summary: “ally's inner thoughts and intimate experiences are revealed as she creates a list of people she has slept with, leading to personal reflections and revelations”

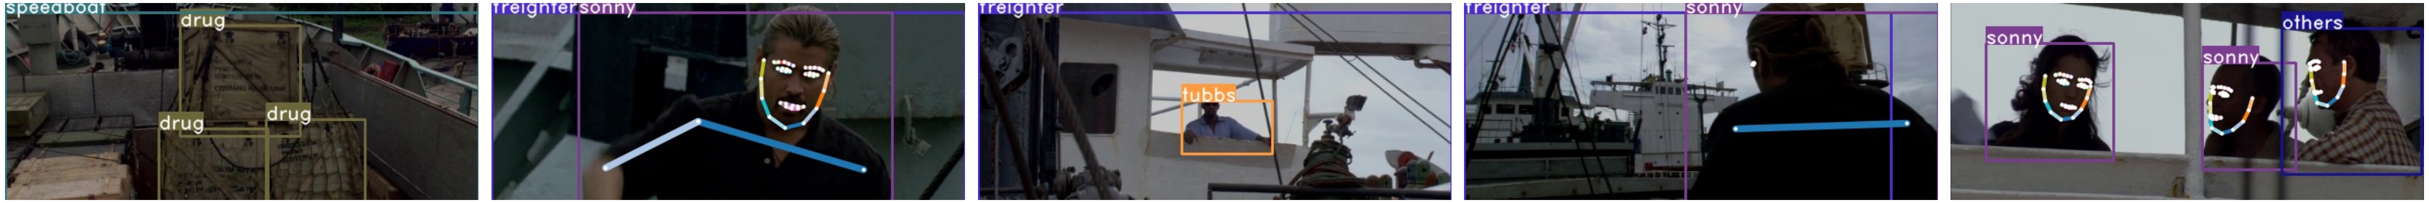


Sonny and Tubbs and the rest of the squad (except Trudy) begin loading drugs from a freighter onto some speedboats.

'title': "undercover operation: sonny and tubbs' drug seizure",
'genre': 'crime and action',
'scene': 'freighter and speedboats’,
'summary': 'sonny, tubbs, and the rest of the squad embark on a risky operation to seize drugs from a freighter’,
'expressions': 'determination and focus',

debug_v2_vis_movienet_storyboard/30

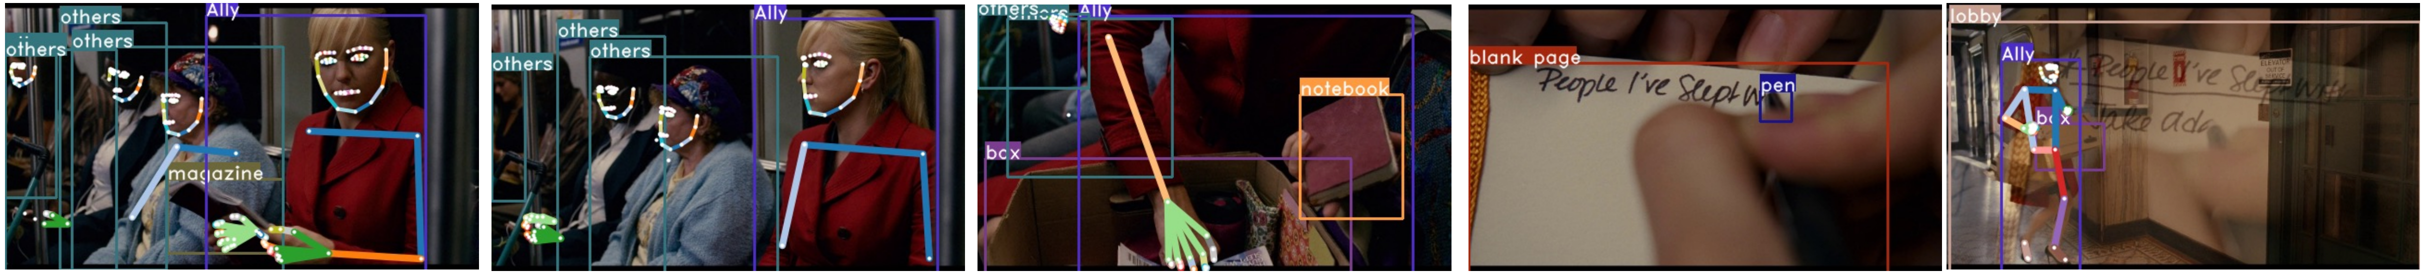


['Ally sets the magazine aside', 'then bites her lip and shifts her calculating gaze.', 'Ally reaches into the box and pulls out a small notebook and pen.', 'Glancing around, Ally opens it and heads a blank page with the words "People I\'ve Slept With. ".', "Now as Ally enters her apartment building's lobby, her list fades into view.", 'Finding the elevator out of service, Ally heads up the winding rectangular staircase.', 'Now a wall in her apartment shows her shadow as Ally undresses.', 'Wearing only panties, Ally scampers across our view.', 'Now Ally showers with the bathroom door open.', 'Ally steps out of the shower, obscured by steam.’]

'title': "intimate confessions: ally's secret list", 'genre':

debug_v2_vis_lsmdc_storyboard/17
